# Supplementary material for: Ab initio Ultrafast Spin Dynamics in Solids
Source: arXiv:2012.08711 source file (2021-09-30)
Supplement: Supplementary file 1 [file SI.pdf]

# Supplemental Material for: *Ab initio* Ultrafast Spin Dynamics in Solids


Junqing Xu[c],[1] Adela Habib[c],[2] Ravishankar Sundararaman[b],[3] and Yuan Ping[a1]

[1] *Department of Chemistry and Biochemistry, University of California, Santa Cruz, CA 95064, USA*
[2] *Department of Physics, Applied Physics and Astronomy, Rensselaer Polytechnic Institute, 110 8th Street, Troy, New York 12180, USA*
[3] *Department of Materials Science and Engineering, Rensselaer Polytechnic Institute, 110 8th Street, Troy, New York 12180, USA*



(Dated: June 25, 2021)


## I. ELECTRONIC BAND STRUCTURE WITH WANNIERIZATION

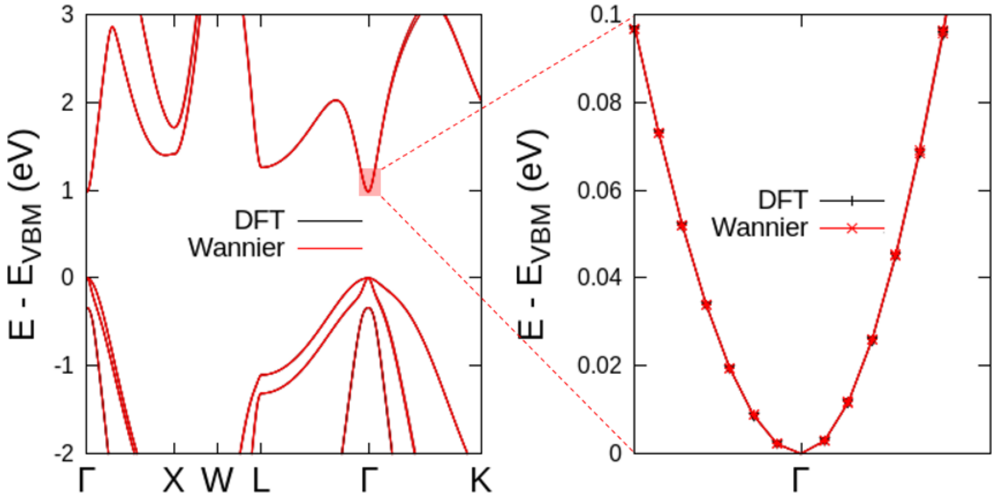


FIG. S1. Wannier-interpolated band structure of GaAs compared with that directly calculated by DFT in a wide energy range (left panel) and close to CBM (right panel).

Figure S1 shows that our Wannier-interpolated band structures fit perfectly with those directly calculated by density functional theory (DFT). This ensures the high quality of the Wannierization, which is crucial to obtaining accurate lifetime results.


[c] JX and AH contributed equally to this work.
[b] sundar@rpi.edu
[a] yuanping@ucsc.edu

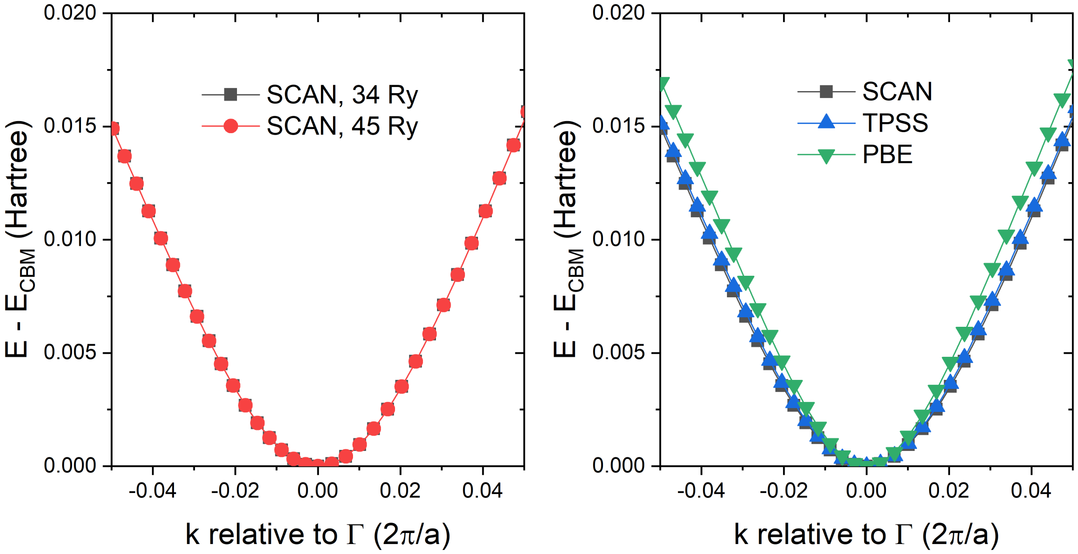


FIG. S2. Calculated dispersion of the lowest conduction band of GaAs around CBM with different wavefunction cutoff energies (left panel) and three exchange-correlation functionals - SCAN[1], TPSS[2] and PBE[3] (right panel). For $x$ axis, negative and positive values correspond to k points along $L-\Gamma$ and $\Gamma-K$ high-symmetry lines, respectively.

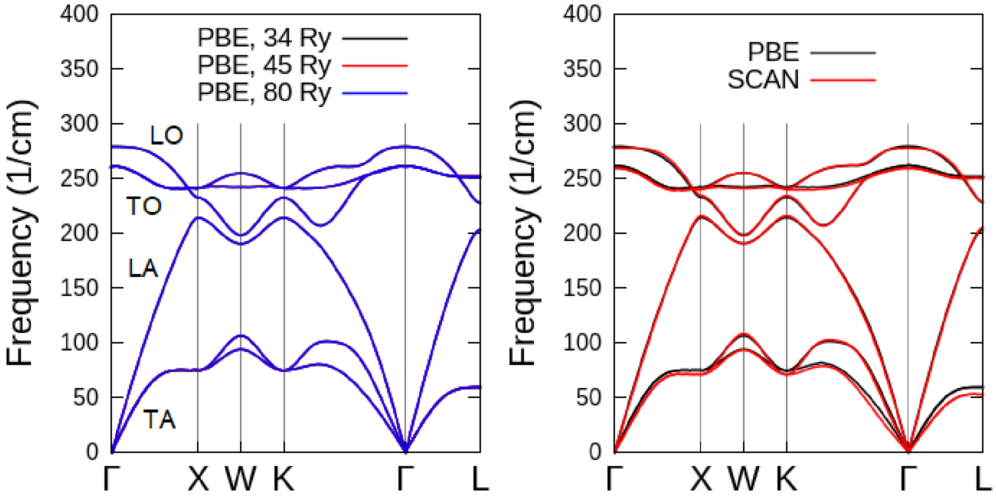


FIG. S3. Phonon dispersion of GaAs with different wavefunction cutoff energies (left panel) and exchange-correlation functionals (right panel). TA, LA, TO and LO represent transverse acoustic, longitudinal acoustic, transverse optical and longitudinal optical modes, respectively.

## II. ENERGY CUTOFF CONVERGENCE AND FUNCTIONAL DEPENDENCE OF ELECTRON AND PHONON DISPERSIONS

For lifetime calculations of n-type semiconductor, dispersion of conduction bands around band edges is rather important. Thus in Fig. S2, we compare the calculated dispersion around conduction band minimum (CBM) of GaAs with different wavefunction cutoff energies and exchange-correlation functionals. It shows that with the chosen norm-conserving pseudopotentials, cutoff energy 34 Ry is enough for convergence. Compared with PBE functional, the effective masses at CBM by SCAN[1] and TPSS[2] are slightly larger (as the dispersion shown in the right panel of Fig. S2). We obtained $0.054m_e$ by SCAN, in good agreement with the experimental value - $0.067m_e$[4].

From Fig. S3, it can be seen that cutoff energy 34 Ry is high enough to converge the phonon dispersion, and SCAN functional gives similar phonon dispersion compared with PBE functional.

We further tested another meta-GGA "MVS" functional[5]. It leads to an effective mass of about $0.07m_e$, even closer to experimental value $0.067m_e$ compared with other exchange-correlation functionals we tested. But the resulting

spin lifetimes are quite similar to those obtained with SCAN functional and the differences are within 10%. This indicates that our theoretical results are relatively robust against the choice of the functional.

## III. CONVERGENCE TESTS FOR REAL-TIME DYNAMICS SIMULATIONS

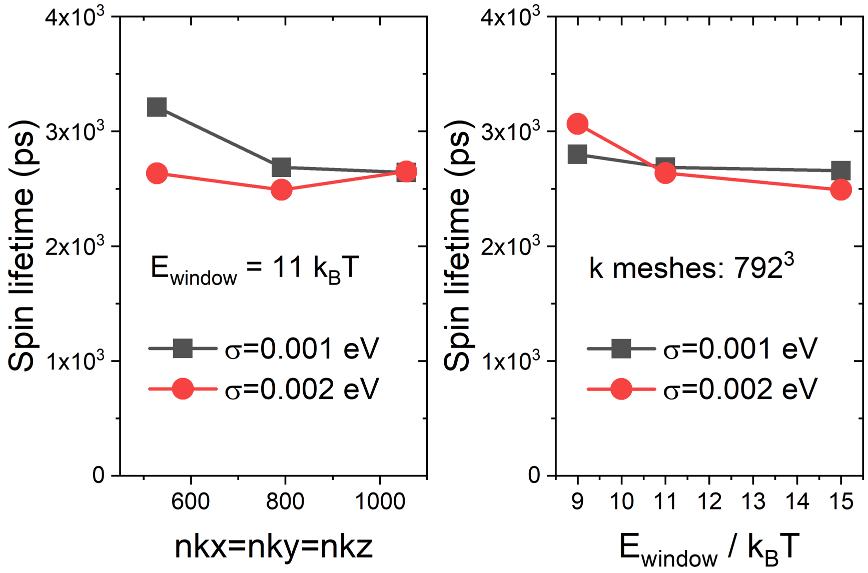


FIG. S4. k-point and energy-window convergence tests for spin lifetime of GaAs at 30 K with $n_i = 2 \times 10^{16}$ cm$^{-3}$ with two smearing parameters $\sigma$ comparable to $k_BT$. For a given $E_{window}$, we will only include electronic states within the energy window $[\epsilon_{CBM},\epsilon_{CBM} + E_{window}]$ during the scattering processes.

In Fig. S4, we show k-point (left panel) and energy-window (right panel) convergence tests at a low temperature - 30 K with two smearing values for energy conservation comparable to $k_BT$. We find that extremely fine k meshes are necessary ($\sim 800^3$), but a reasonably large energy window ($\sim 10k_BT$) for selecting electronic states is enough. Therefore, at 30 K, we use k meshes $792\times792\times792$ and the energy window about $[\epsilon_{CBM}, \max(\epsilon_{CBM}, \mu_{max})+10k_BT]$, where $\mu_{max}$ is maximum of the chemical potentials used at a given temperature. At all temperatures, we have tested the convergence carefully to make sure the convergence of spin lifetimes within 20%.

## IV. THE TREATMENT OF SCATTERING PROCESSES FOR HOLES IN $n$-GaAs

For $n$-GaAs, it is unnecessary to treat scattering processes of holes exactly. This is because: (i) When $\rho$ is initialized by a test magnetic field (see main text Sec. II), the dynamics of holes will be irrelevant as hole concentration is negligible; (ii) When $\rho$ is initialized by a pump pulse, there are some holes being excited. But since the time scale of hole spin relaxation, $\sim$ 110 fs at 300 K[6], is much faster than the time scale of the Kerr rotation, the hole scattering processes should have little effects on global Kerr-rotation or spin dynamics. Therefore, when the pump process is active, the dynamics of holes are described approximately by assuming the time derivative of the hole density matrix satisfies $d\rho/dt = -\left(\rho - \rho^{\text{eq}}\right)/\tau_{\text{hole}}$ with $\tau_{\text{hole}}$=110 fs at 300 K. And we have confirmed the real-time dynamics is insensitive to the specific choice of $\tau_{\text{hole}}$.

## V. ELECTRONIC BAND STRUCTURE OF FEW-LAYER $WSe_2$

Figure S5 shows band structure of monolayer $WSe_2$. It can be seen that states around band edges are highly spin polarized along z, and the SOC-induced band splittings at high-symmetry point $K$ are about 465 and 37 meV for valence and conduction bands, respectively.

Figure S6 shows band structures of inversion-symmetric bilayer $WSe_2$ with different strains. It can be seen that valence band maximum is located at $\Gamma$ without a strain, which is consistent with the theoretical study in Ref. 7 from

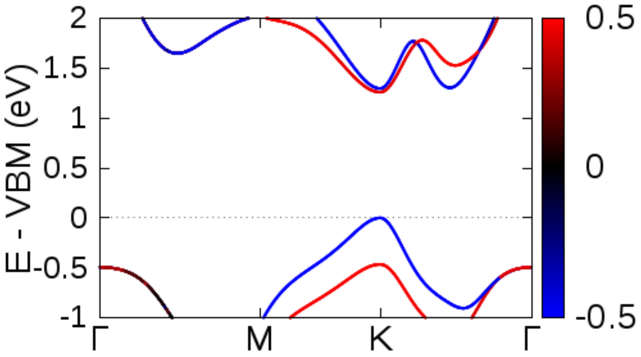


FIG. S5. Band structure of monolayer $WSe_2$. Color represent spin expectation value along $z$ direction $s^{\mathrm{exp}}_{\mathbf{k},z}$.

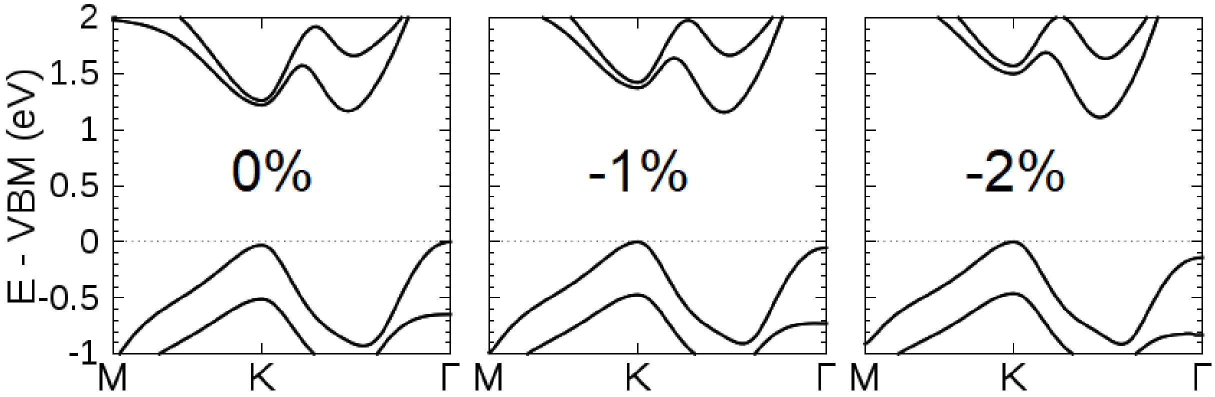


FIG. S6. Band structures of inversion-symmetric bilayer $WSe_2$ (AB stacking, see main text Fig.6) with different strains. A negative strain means a compressive strain.

both DFT and GW calculations and experimental study in Ref. 8, but valence band maximum switches to $K$ with a compressive strain.

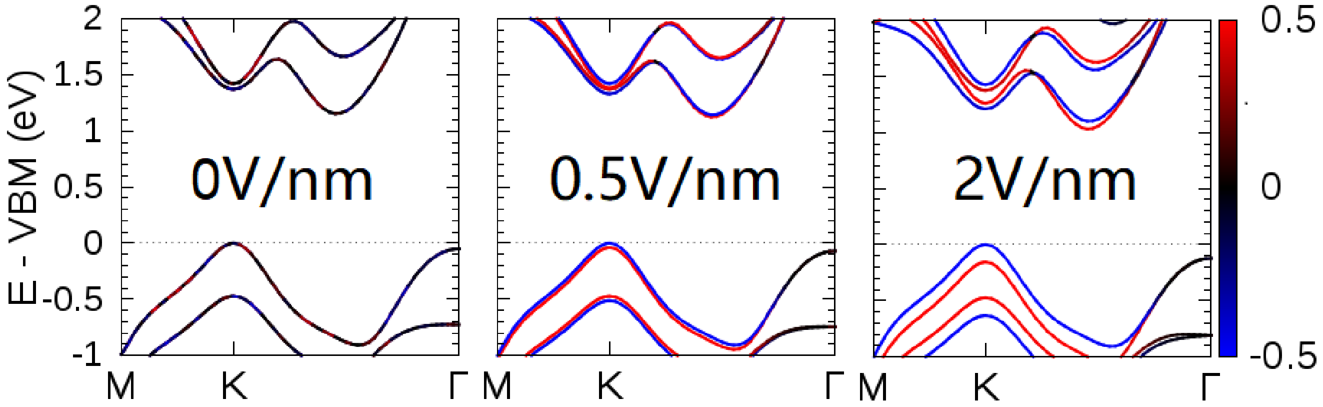


FIG. S7. Band structures of 1% compressed bilayer $WSe_2$ with different $E_z$. Color represent spin expectation value along $z$ direction $s^{\mathrm{exp}}_{\mathbf{k},i}$.

Figure S7 shows band structures of 1% compressed bilayer $WSe_2$ with under different $E_z$. Under zero $E_z$, bands of bilayer $WSe_2$ will form two-fold (Kramers) degenerate pairs due to inversion symmetry. It can be seen that under a finite electric field, the band degeneracy is lifted except at $\Gamma$ and the band splitting increases with $E_z$. Moreover, under finite $E_z$, states around $K$ are highly spin-polarized consistent with the schematic diagram of the band structure of bilayer $WSe_2$ in Fig. 7a.

## VI. PHONON DISPERSION OF FEW-LAYER $WSe_2$

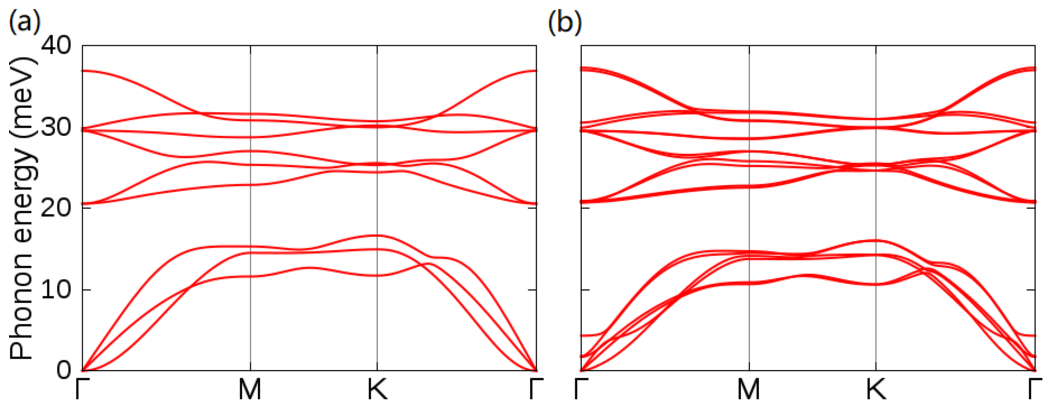


FIG. S8. Phonon dispersion of (a) monolayer and (b) bilayer $WSe_2$.

Figure S8 shows phonon dispersions of monolayer and bilayer $WSe_2$. The phonon dispersion of the bilayer is rather similar to monolayer except in the low frequency region and at $\mathbf{q}$ points close to $\Gamma$.

## VII. ELECTRON-IMPURITY MATRIX ELEMENTS OF DIFFERENT TYPES OF NEUTRAL IMPURITIES IN MONOLAYER $WSe_2$

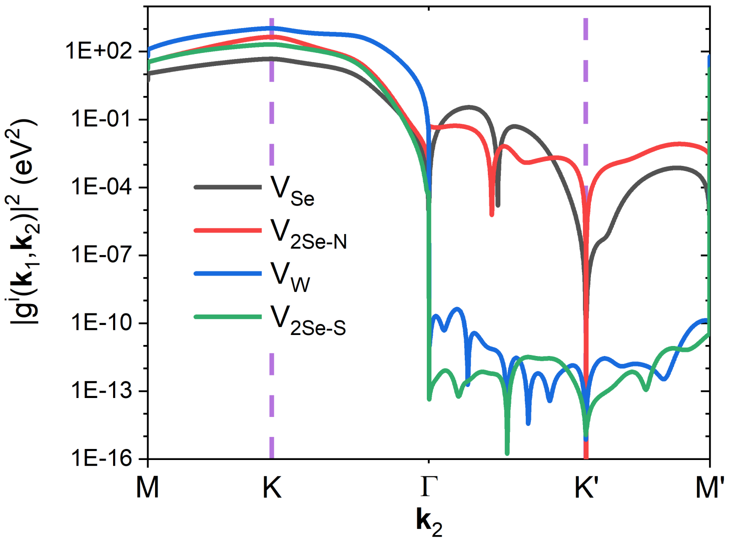


FIG. S9. The squares of electron-impurity matrix elements $|g^i_{\mathbf{k_1 n_1 k_2 n_2}}|^2$ between fixed state $(\mathbf{k_1}, \mathbf{n_1})$ and state $(\mathbf{k_2}, \mathbf{n_2})$ along high-symmetry lines of four types of neutral impurities in monolayer $WSe_2$. $\mathbf{k}$ and $n$ are wave vector and band index, respectively. $n_1$ and $n_2$ are both the highest valence band. $\mathbf{k_1}$ is fixed at (0.333780,0.332440) a little away from $K$.

In Fig. S9, we compare electron-impurity matrix elements of four types of neutral impurities in monolayer $WSe_2$ between fixed state $(k_1, n_1)$ and state $(k_2, n_2)$ along high-symmetry lines, where $n_1$ and $n_2$ are both the highest valence band and $k_1$ is fixed at (0.333780,0.332440) a little away from $K$. First we can see that intravalley spin-conserving scattering ($k_2$ at $K$) is much stronger than intervalley spin-flip scattering ($k_2$ at $K'$), which is expected. For holes of monolayer $WSe_2$, intravalley /intervalley scattering determines carrier/spin dynamics. From Fig. S9, we find that although the effects of different impurities on carrier and spin dynamics are all different, the differences of their effects on spin dynamics are much stronger. For intervalley spin-flip scattering, we have $V_{2Se-N} \gg V_{Se} \gg V_W \sim V_{2Se-S}$, consistent with the strength of their effects on spin relaxation times as shown in Fig. 6.

## VIII. ELECTRON-PHONON MATRIX ELEMENTS OF BILAYER $WSe_2$

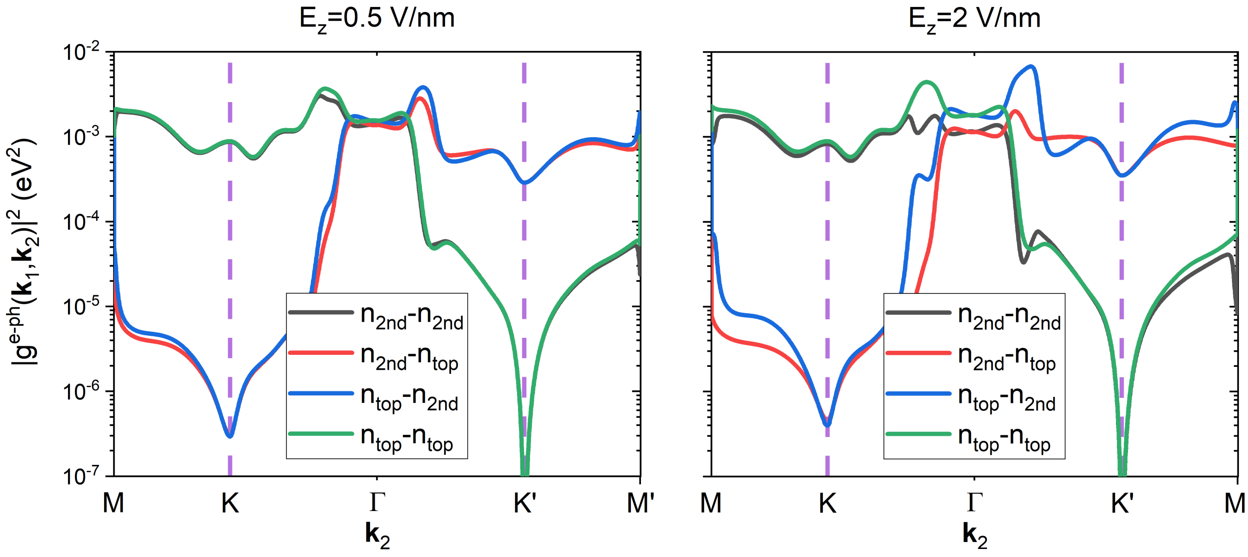


FIG. S10. The modue square of electron-phonon matrix elements $|g^{\mathrm{e-ph}}|^2$ of 1% compressed bilayer $WSe_2$ under (left panel) 0.5 and (right panel) 2 V/nm between $(\mathbf{k}_1, n_1)$ and state $(\mathbf{k}_2, n_2)$ along high-symmetry lines. $\mathbf{k}$ and $n$ are wave vector and band index, respectively. $\mathbf{k_1}$ is fixed at (0.333780,0.332440) a little away from $K$. The red line represents $|g^{\mathrm{e-ph}}|^2$ between the second valence band ($n_1 = n_{\mathrm{2nd}}$) and the top valence band ($n_2 = n_{\mathrm{top}}$). Similarly, other lines represent $|g^{\mathrm{e-ph}}|^2$ between two corresponding bands.

Since at 50 K, e-ph scattering is more important than e-i scattering, here we will show the squares of e-ph matrix elements $|g^{\mathrm{e-ph}}|^2$ of bilayer $WSe_2$ for understanding better ultrafast dynamics in the bilayer.

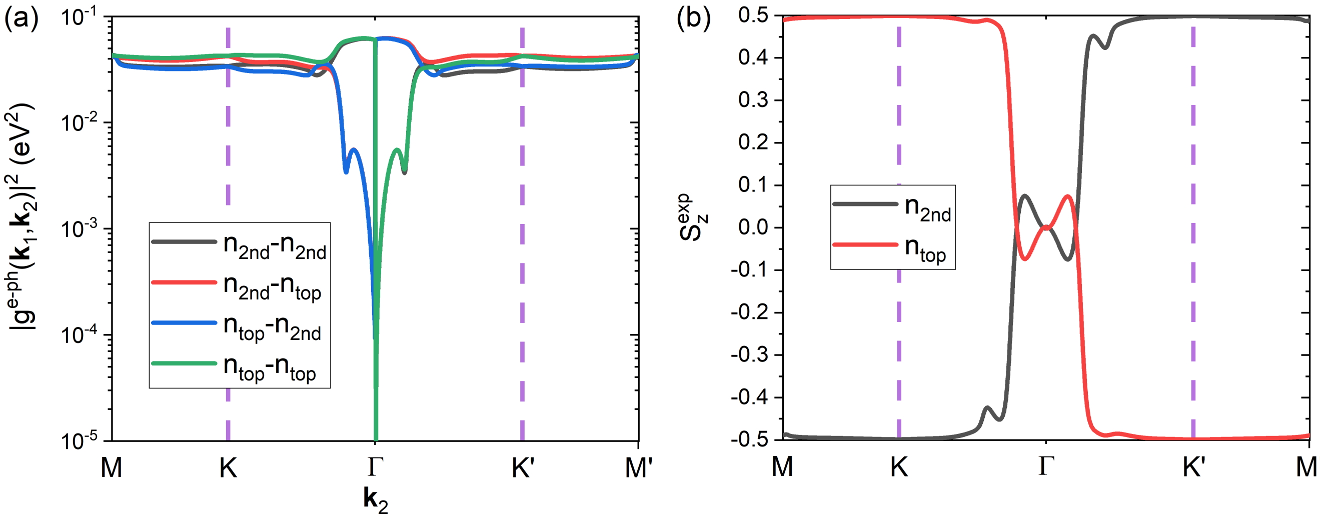


FIG. S11. (a) The module square of electron-phonon matrix elements $|g^{\mathrm{e-ph}}|^2$ of 1% compressed bilayer $WSe_2$ under $E_z$=2 V/nm between $(\mathbf{k}_1, n_1)$ and state $(\mathbf{k}_2, n_2)$ along high-symmetry lines. $\mathbf{k}$ and $n$ are wave vector and band index, respectively. $\mathbf{k_1}$ is fixed at (0.0014,0.0014) a little away from $\Gamma$. The red line represents $|g^{\mathrm{e-ph}}|^2$ between the second valence band ($n_1 = n_{\mathrm{2nd}}$) and the top valence band ($n_2 = n_{\mathrm{top}}$). Similarly, other lines represent $|g^{\mathrm{e-ph}}|^2$ between two corresponding bands. (b) Spin expectation value $s_z^{\mathrm{exp}}$ of two top valence bands along high-symmetry lines of 1% compressed bilayer $WSe_2$ under $E_z$=2 V/nm.

From S10 and considering the band structure of compressed bilayer $WSe_2$ shown in Fig. 7 and S7, we find that for compressed bilayer $WSe_2$ under finite $E_z$, (i) $|g^{\mathrm{e-ph}}|^2$ under different $E_z$ are similar. (ii) $|g^{\mathrm{e-ph}}|^2$ between $\Gamma$ and $K$ valleys are about 3 times larger than that intervalley (and interlayer) spin conserving $|g^{\mathrm{e-ph}}|^2$ between $K$ and $K'$

valleys (red and blue lines and around $K'$), and (iii) intervalley (and interlayer) spin conserving $|g^{\mathrm{e-ph}}|^2$ between $K$ and $K'$ valleys (red and blue lines and around $K'$) are much larger than both intervalley (between $K$ and $K'$, black and green lines and around $K'$) and intravalley (within $K$ or $K'$, red and blue lines and around $K$) spin-flip $|g^{\mathrm{e-ph}}|^2$.

From S11, we can see that $|g^{\mathrm{e-ph}}|^2$ of $\Gamma - K$ and $\Gamma - K'$ transitions are quite similar. This is partly because: electron spins at $\Gamma$ valleys are not highly polarized along $z$ direction but mostly along in-plane directions so that the transitions between $\Gamma$ and $K/K'$ will not be suppressed/enhanced due to opposite/same spin directions.

## IX. HOLE-DENSITY DEPENDENCE OF SPIN LIFETIME OF MONOLAYER $WSe_2$

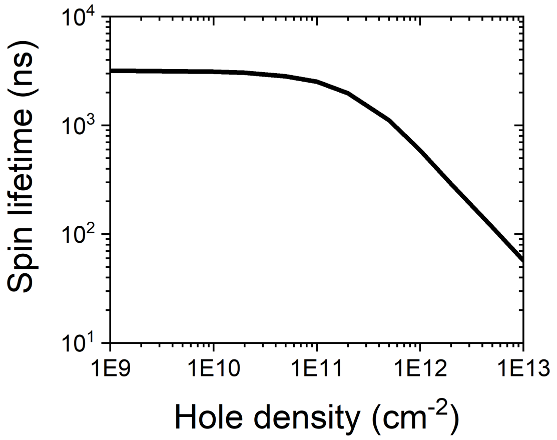


FIG. S12. Spin lifetimes of resident holes of monolayer $WSe_2$ with $8\times10^9$ cm$^{-2}$ $V_{2\mathrm{Se-N}}$ at 15 K as a function of hole density.

From Fig. S12, it is found that spin lifetimes of resident holes of monolayer $WSe_2$ are highly sensitive to hole density, in good agreement with experimental observations[9].

[1] J. Sun, A. Ruzsinszky, and J. P. Perdew, "Strongly Constrained and Appropriately Normed Semilocal Density Functional," Phys. Rev. Lett. **115**, 036402 (2015).

[2] J. Tao, J. P. Perdew, V. N. Staroverov, and G. E. Scuseria, "Climbing the Density Functional Ladder: Nonempirical Meta–Generalized Gradient Approximation Designed for Molecules and Solids," Phys. Rev. Lett. **91**, 146401 (2003).

[3] J. P. Perdew, K. Burke, and M. Ernzerhof, "Generalized Gradient Approximation Made Simple," Phys. Rev. Lett. **77**, 3865 (1996).

[4] O. Madelung, *Semiconductors* (Springer, 1987).

[5] J. Sun, J. P. Perdew, and A. Ruzsinszky, "Semilocal density functional obeying a strongly tightened bound for exchange," Proc. Natl. Acad. Sci. **112**, 685–689 (2015).

[6] D. J. Hilton and C. L. Tang, "Optical Orientation and Femtosecond Relaxation of Spin-Polarized Holes in GaAs," Phys. Rev. Lett. **89**, 146601 (2002).

[7] H. Kim and H. J. Choi, "Thickness dependence of work function, ionization energy, and electron affinity of Mo and W dichalcogenides from DFT and GW calculations," Phys. Rev. B **103**, 085404 (2021).

[8] W. Zhao, R. M. Ribeiro, M. Toh, A. Carvalho, C. Kloc, A. H. Castro Neto, and G. Eda, "Origin of indirect optical transitions in few-layer MoS2, WS2, and WSe2," Nano Lett. **13**, 5627–5634 (2013).

[9] J. Li, M. Goryca, K. Yumigeta, H. Li, S. Tongay, and S. A. Crooker, "Valley relaxation of resident electrons and holes in a monolayer semiconductor: Dependence on carrier density and the role of substrate-induced disorder," Phys. Rev. Mater. **5**, 044001 (2021).
